# Supplementary material for: Pandemics Depress the Economy, Public Health Interventions Do Not: Evidence from the 1918 Flu
Source: arXiv:2207.11636 source file (2022-07-24)
Supplement: Supplementary file 4 [file 2_reg_W_cat_npi.tex]

&         (1)   &         (2)   &         (3)   &         (4)   &         (5)   &         (6)   \\
 \cmidrule(lr){1-7}  $NPI \ Intensity_c \times Post_{t}$&       0.001   &       0.000   &               &               &               &               \\
                    &     (0.001)   &     (0.001)   &               &               &               &               \\
$NPI \ Speed_c \times  Post_{t}$&               &               &      -0.007   &      -0.002   &               &               \\
                    &               &               &     (0.008)   &     (0.008)   &               &               \\
 $  High \ NPI_c \times  Post_{t}$&               &               &               &               &       0.101   &      -0.041   \\
                    &               &               &               &               &     (0.126)   &     (0.136)   \\
\cmidrule{1-7}
\cmidrule(lr){1-7} Within \RSq&        0.01   &        0.05   &        0.01   &        0.05   &        0.00   &        0.05   \\
Observations        &         398   &         398   &         398   &         398   &         398   &         398   \\
Number of cities    &          27   &          27   &          27   &          27   &          27   &          27   \\
\Oster              &           .   &     -.00027   &           .   &     -.00079   &           .   &       -.088   \\
Baseline controls   &           -   &         Yes   &           -   &         Yes   &           -   &         Yes   \\
    \bottomrule
