# Supplementary material for: Pandemics Depress the Economy, Public Health Interventions Do Not: Evidence from the 1918 Flu
Source: arXiv:2207.11636 source file (2022-07-24)
Supplement: Supplementary file 7 [file mortality_allcause_edr_drop_west.tex]

&         (1)   &         (2)   &         (3)   &         (4)   &         (5)   &         (6)   &         (7)   &         (8)   &         (9)   \\
\cmidrule{1-10}Intensity&       -1.45** &       -1.05*  &       -0.60   &               &               &               &               &               &               \\
                    &      (0.57)   &      (0.57)   &      (0.57)   &               &               &               &               &               &               \\
Speed               &               &               &               &       -4.16   &       -4.82** &       -3.58   &               &               &               \\
                    &               &               &               &      (3.23)   &      (2.06)   &      (2.32)   &               &               &               \\
High NPI            &               &               &               &               &               &               &     -142.51***&     -114.96***&      -98.00** \\
                    &               &               &               &               &               &               &     (42.38)   &     (41.60)   &     (46.66)   \\
\cmidrule{1-10}
\RSq                &        0.13   &        0.55   &        0.61   &        0.04   &        0.53   &        0.62   &        0.17   &        0.58   &        0.63   \\
Observations        &          39   &          39   &          39   &          39   &          39   &          39   &          39   &          39   &          39   \\
\Oster              &           .   &         -.9   &        -.28   &           .   &          -5   &        -3.4   &           .   &        -103   &         -80   \\
Baseline controls   &           -   &         Yes   &         Yes   &           -   &         Yes   &         Yes   &           -   &         Yes   &         Yes   \\
   \bottomrule
