# Supplementary material for: Pandemics Depress the Economy, Public Health Interventions Do Not: Evidence from the 1918 Flu
Source: arXiv:2207.11636 source file (2022-07-24)
Supplement: Supplementary file 9 [file mortality_allcause_peak_value_drop_west.tex]

&         (1)   &         (2)   &         (3)   &         (4)   &         (5)   &         (6)   &         (7)   &         (8)   &         (9)   \\
\cmidrule{1-10}Intensity&       -0.59***&       -0.56***&       -0.21   &               &               &               &               &               &               \\
                    &      (0.14)   &      (0.17)   &      (0.18)   &               &               &               &               &               &               \\
Speed               &               &               &               &       -0.99   &       -1.14   &       -0.43   &               &               &               \\
                    &               &               &               &      (1.04)   &      (0.99)   &      (0.79)   &               &               &               \\
High NPI            &               &               &               &               &               &               &      -57.66***&      -59.65***&      -37.26*  \\
                    &               &               &               &               &               &               &     (12.11)   &     (15.43)   &     (19.56)   \\
\cmidrule{1-10}
\RSq                &        0.21   &        0.55   &        0.65   &        0.02   &        0.41   &        0.64   &        0.26   &        0.61   &        0.68   \\
Observations        &          39   &          39   &          39   &          39   &          39   &          39   &          39   &          39   &          39   \\
\Oster              &           .   &        -.55   &       -.047   &           .   &        -1.2   &        -.26   &           .   &         -61   &         -27   \\
Baseline controls   &           -   &         Yes   &         Yes   &           -   &         Yes   &         Yes   &           -   &         Yes   &         Yes   \\
   \bottomrule
