# Supplementary material for: Pandemics Depress the Economy, Public Health Interventions Do Not: Evidence from the 1918 Flu
Source: arXiv:2207.11636 source file (2022-07-24)
Supplement: Supplementary file 11 [file mortality_ip_edr_details_drop_west.tex]

&         (1)   &         (2)   &         (3)   &         (4)   &         (5)   &         (6)   &         (7)   &         (8)   &         (9)   \\
\cmidrule{1-10} \NPIIntensity&        -1.3** &        -1.1** &        -0.6   &               &               &               &               &               &               \\
                    &       (0.5)   &       (0.5)   &       (0.5)   &               &               &               &               &               &               \\
\NPISpeed           &               &               &               &        -3.1   &        -3.8** &        -2.4   &               &               &               \\
                    &               &               &               &       (2.6)   &       (1.7)   &       (1.7)   &               &               &               \\
\HighNPI            &               &               &               &               &               &               &      -136.0***&      -114.2***&       -87.5*  \\
                    &               &               &               &               &               &               &      (38.7)   &      (39.1)   &      (45.3)   \\
1917 I\&P mortality (per 100k)&               &         1.9***&         1.9***&               &         2.0***&         1.8***&               &         1.8***&         1.8***\\
                    &               &       (0.4)   &       (0.4)   &               &       (0.4)   &       (0.4)   &               &       (0.4)   &       (0.5)   \\
Longitude           &               &               &         7.3** &               &               &         8.2***&               &               &         5.4*  \\
                    &               &               &       (3.1)   &               &               &       (2.8)   &               &               &       (3.1)   \\
Illiteracy          &               &               &        -3.5   &               &               &         1.3   &               &               &        -3.6   \\
                    &               &               &       (8.4)   &               &               &       (8.6)   &               &               &       (8.1)   \\
Medium coal-fired capacity&               &               &        46.6   &               &               &        53.1   &               &               &        81.1   \\
                    &               &               &      (58.6)   &               &               &      (54.1)   &               &               &      (67.0)   \\
High coal-fired capacity&               &               &        32.2   &               &               &        25.4   &               &               &        50.0   \\
                    &               &               &      (54.9)   &               &               &      (52.1)   &               &               &      (63.0)   \\
\cmidrule{1-10}
\RSq                &        0.15   &        0.58   &        0.64   &        0.03   &        0.53   &        0.64   &        0.21   &        0.61   &        0.66   \\
Observations        &          39   &          39   &          39   &          39   &          39   &          39   &          39   &          39   &          39   \\
\Oster              &           .   &        -.98   &        -.28   &           .   &          -4   &        -2.2   &           .   &        -104   &         -66   \\
Baseline controls   &           -   &         Yes   &         Yes   &           -   &         Yes   &         Yes   &           -   &         Yes   &         Yes   \\
   \bottomrule
