# Supplementary material for: Pandemics Depress the Economy, Public Health Interventions Do Not: Evidence from the 1918 Flu
Source: arXiv:2207.11636 source file (2022-07-24)
Supplement: Supplementary file 12 [file mortality_ip_edr_drop_west.tex]

&         (1)   &         (2)   &         (3)   &         (4)   &         (5)   &         (6)   &         (7)   &         (8)   &         (9)   \\
\cmidrule{1-10}Intensity&       -1.31** &       -1.08** &       -0.57   &               &               &               &               &               &               \\
                    &      (0.51)   &      (0.47)   &      (0.53)   &               &               &               &               &               &               \\
Speed               &               &               &               &       -3.11   &       -3.76** &       -2.43   &               &               &               \\
                    &               &               &               &      (2.64)   &      (1.73)   &      (1.75)   &               &               &               \\
High NPI            &               &               &               &               &               &               &     -136.05***&     -114.21***&      -87.54*  \\
                    &               &               &               &               &               &               &     (38.68)   &     (39.06)   &     (45.30)   \\
\cmidrule{1-10}
\RSq                &        0.15   &        0.58   &        0.64   &        0.03   &        0.53   &        0.64   &        0.21   &        0.61   &        0.66   \\
Observations        &          39   &          39   &          39   &          39   &          39   &          39   &          39   &          39   &          39   \\
\Oster              &           .   &        -.98   &        -.28   &           .   &          -4   &        -2.2   &           .   &        -104   &         -66   \\
Baseline controls   &           -   &         Yes   &         Yes   &           -   &         Yes   &         Yes   &           -   &         Yes   &         Yes   \\
   \bottomrule
