# Supplementary material for: Pandemics Depress the Economy, Public Health Interventions Do Not: Evidence from the 1918 Flu
Source: arXiv:2207.11636 source file (2022-07-24)
Supplement: Supplementary file 14 [file mortality_ip_peak_value_details_drop_west.tex]

&         (1)   &         (2)   &         (3)   &         (4)   &         (5)   &         (6)   &         (7)   &         (8)   &         (9)   \\
\cmidrule{1-10} \NPIIntensity&        -0.6***&        -0.6***&        -0.2   &               &               &               &               &               &               \\
                    &       (0.1)   &       (0.2)   &       (0.2)   &               &               &               &               &               &               \\
\NPISpeed           &               &               &               &        -0.9   &        -1.0   &        -0.4   &               &               &               \\
                    &               &               &               &       (0.9)   &       (1.0)   &       (0.8)   &               &               &               \\
\HighNPI            &               &               &               &               &               &               &       -54.3***&       -56.8***&       -34.7*  \\
                    &               &               &               &               &               &               &      (11.1)   &      (14.7)   &      (19.3)   \\
1917 I\&P mortality (per 100k)&               &         0.4*  &         0.3   &               &         0.4** &         0.3   &               &         0.3   &         0.3   \\
                    &               &       (0.2)   &       (0.2)   &               &       (0.2)   &       (0.2)   &               &       (0.2)   &       (0.2)   \\
Longitude           &               &               &         3.1***&               &               &         3.7***&               &               &         2.3** \\
                    &               &               &       (1.1)   &               &               &       (0.9)   &               &               &       (1.1)   \\
Illiteracy          &               &               &         2.6   &               &               &         4.1   &               &               &         2.4   \\
                    &               &               &       (3.4)   &               &               &       (2.8)   &               &               &       (3.1)   \\
Medium coal-fired capacity&               &               &        -3.6   &               &               &        -4.4   &               &               &        10.2   \\
                    &               &               &      (19.3)   &               &               &      (18.3)   &               &               &      (20.9)   \\
High coal-fired capacity&               &               &       -21.5   &               &               &       -24.4   &               &               &       -14.2   \\
                    &               &               &      (18.5)   &               &               &      (18.5)   &               &               &      (18.8)   \\
\cmidrule{1-10}
\RSq                &        0.23   &        0.52   &        0.62   &        0.02   &        0.34   &        0.61   &        0.28   &        0.57   &        0.66   \\
Observations        &          39   &          39   &          39   &          39   &          39   &          39   &          39   &          39   &          39   \\
\Oster              &           .   &        -.55   &       -.042   &           .   &          -1   &        -.19   &           .   &         -58   &         -24   \\
Baseline controls   &           -   &         Yes   &         Yes   &           -   &         Yes   &         Yes   &           -   &         Yes   &         Yes   \\
   \bottomrule
