# Supplementary material for: Pandemics Depress the Economy, Public Health Interventions Do Not: Evidence from the 1918 Flu
Source: arXiv:2207.11636 source file (2022-07-24)
Supplement: Supplementary file 15 [file mortality_ip_peak_value_drop_west.tex]

&         (1)   &         (2)   &         (3)   &         (4)   &         (5)   &         (6)   &         (7)   &         (8)   &         (9)   \\
\cmidrule{1-10}Intensity&       -0.56***&       -0.55***&       -0.21   &               &               &               &               &               &               \\
                    &      (0.13)   &      (0.16)   &      (0.18)   &               &               &               &               &               &               \\
Speed               &               &               &               &       -0.90   &       -1.01   &       -0.36   &               &               &               \\
                    &               &               &               &      (0.95)   &      (0.96)   &      (0.75)   &               &               &               \\
High NPI            &               &               &               &               &               &               &      -54.35***&      -56.85***&      -34.67*  \\
                    &               &               &               &               &               &               &     (11.10)   &     (14.74)   &     (19.30)   \\
\cmidrule{1-10}
\RSq                &        0.23   &        0.52   &        0.62   &        0.02   &        0.34   &        0.61   &        0.28   &        0.57   &        0.66   \\
Observations        &          39   &          39   &          39   &          39   &          39   &          39   &          39   &          39   &          39   \\
\Oster              &           .   &        -.55   &       -.042   &           .   &          -1   &        -.19   &           .   &         -58   &         -24   \\
Baseline controls   &           -   &         Yes   &         Yes   &           -   &         Yes   &         Yes   &           -   &         Yes   &         Yes   \\
   \bottomrule
