# Supplementary material for: Pandemics Depress the Economy, Public Health Interventions Do Not: Evidence from the 1918 Flu
Source: arXiv:2207.11636 source file (2022-07-24)
Supplement: Supplementary file 16 [file mortality_markel_edr_details_drop_west.tex]

&         (1)   &         (2)   &         (3)   &         (4)   &         (5)   &         (6)   &         (7)   &         (8)   &         (9)   \\
\cmidrule{1-10} \NPIIntensity&        -1.5***&        -1.2** &        -0.7   &               &               &               &               &               &               \\
                    &       (0.5)   &       (0.5)   &       (0.5)   &               &               &               &               &               &               \\
\NPISpeed           &               &               &               &        -3.8   &        -4.5** &        -2.9   &               &               &               \\
                    &               &               &               &       (2.8)   &       (1.8)   &       (1.9)   &               &               &               \\
\HighNPI            &               &               &               &               &               &               &      -150.3***&      -128.0***&       -97.4*  \\
                    &               &               &               &               &               &               &      (39.7)   &      (39.1)   &      (47.9)   \\
1917 I\&P mortality (per 100k)&               &         2.0***&         2.0***&               &         2.1***&         1.9***&               &         1.9***&         1.9***\\
                    &               &       (0.3)   &       (0.4)   &               &       (0.4)   &       (0.4)   &               &       (0.4)   &       (0.5)   \\
Longitude           &               &               &         8.2** &               &               &         9.2***&               &               &         6.1*  \\
                    &               &               &       (3.1)   &               &               &       (2.8)   &               &               &       (3.1)   \\
Illiteracy          &               &               &        -4.8   &               &               &         0.7   &               &               &        -4.8   \\
                    &               &               &       (9.0)   &               &               &       (9.2)   &               &               &       (8.6)   \\
Medium coal-fired capacity&               &               &        37.9   &               &               &        45.6   &               &               &        76.0   \\
                    &               &               &      (62.1)   &               &               &      (57.1)   &               &               &      (70.9)   \\
High coal-fired capacity&               &               &        37.6   &               &               &        29.8   &               &               &        57.0   \\
                    &               &               &      (58.0)   &               &               &      (54.7)   &               &               &      (67.4)   \\
\cmidrule{1-10}
\RSq                &        0.16   &        0.59   &        0.66   &        0.04   &        0.54   &        0.66   &        0.23   &        0.63   &        0.69   \\
Observations        &          39   &          39   &          39   &          39   &          39   &          39   &          39   &          39   &          39   \\
\Oster              &           .   &        -1.1   &        -.33   &           .   &        -4.7   &        -2.5   &           .   &        -117   &         -73   \\
Baseline controls   &           -   &         Yes   &         Yes   &           -   &         Yes   &         Yes   &           -   &         Yes   &         Yes   \\
   \bottomrule
