# Supplementary material for: Pandemics Depress the Economy, Public Health Interventions Do Not: Evidence from the 1918 Flu
Source: arXiv:2207.11636 source file (2022-07-24)
Supplement: Supplementary file 17 [file mortality_markel_edr_drop_west.tex]

&         (1)   &         (2)   &         (3)   &         (4)   &         (5)   &         (6)   &         (7)   &         (8)   &         (9)   \\
\cmidrule{1-10}Intensity&       -1.45***&       -1.20** &       -0.65   &               &               &               &               &               &               \\
                    &      (0.52)   &      (0.48)   &      (0.55)   &               &               &               &               &               &               \\
Speed               &               &               &               &       -3.82   &       -4.45** &       -2.85   &               &               &               \\
                    &               &               &               &      (2.78)   &      (1.83)   &      (1.87)   &               &               &               \\
High NPI            &               &               &               &               &               &               &     -150.27***&     -127.99***&      -97.35*  \\
                    &               &               &               &               &               &               &     (39.65)   &     (39.15)   &     (47.89)   \\
\cmidrule{1-10}
\RSq                &        0.16   &        0.59   &        0.66   &        0.04   &        0.54   &        0.66   &        0.23   &        0.63   &        0.69   \\
Observations        &          39   &          39   &          39   &          39   &          39   &          39   &          39   &          39   &          39   \\
\Oster              &           .   &        -1.1   &        -.33   &           .   &        -4.7   &        -2.5   &           .   &        -117   &         -73   \\
Baseline controls   &           -   &         Yes   &         Yes   &           -   &         Yes   &         Yes   &           -   &         Yes   &         Yes   \\
   \bottomrule
