# Supplementary material for: Pandemics Depress the Economy, Public Health Interventions Do Not: Evidence from the 1918 Flu
Source: arXiv:2207.11636 source file (2022-07-24)
Supplement: Supplementary file 18 [file mortality_markel_peak_value_details_drop_west.tex]

&         (1)   &         (2)   &         (3)   &         (4)   &         (5)   &         (6)   &         (7)   &         (8)   &         (9)   \\
\cmidrule{1-10} \NPIIntensity&        -0.6***&        -0.6***&        -0.2   &               &               &               &               &               &               \\
                    &       (0.1)   &       (0.2)   &       (0.2)   &               &               &               &               &               &               \\
\NPISpeed           &               &               &               &        -1.0   &        -1.1   &        -0.4   &               &               &               \\
                    &               &               &               &       (1.0)   &       (1.0)   &       (0.8)   &               &               &               \\
\HighNPI            &               &               &               &               &               &               &       -57.5***&       -59.5***&       -36.1*  \\
                    &               &               &               &               &               &               &      (11.7)   &      (15.3)   &      (18.9)   \\
1917 I\&P mortality (per 100k)&               &         0.4*  &         0.3   &               &         0.5** &         0.3   &               &         0.3   &         0.3   \\
                    &               &       (0.2)   &       (0.2)   &               &       (0.2)   &       (0.2)   &               &       (0.2)   &       (0.2)   \\
Longitude           &               &               &         3.2***&               &               &         3.8***&               &               &         2.4** \\
                    &               &               &       (1.1)   &               &               &       (1.0)   &               &               &       (1.1)   \\
Illiteracy          &               &               &         3.3   &               &               &         5.0*  &               &               &         3.3   \\
                    &               &               &       (3.3)   &               &               &       (2.8)   &               &               &       (3.0)   \\
Medium coal-fired capacity&               &               &         6.8   &               &               &         6.0   &               &               &        21.0   \\
                    &               &               &      (23.2)   &               &               &      (21.7)   &               &               &      (24.8)   \\
High coal-fired capacity&               &               &       -13.5   &               &               &       -16.8   &               &               &        -6.2   \\
                    &               &               &      (21.1)   &               &               &      (20.7)   &               &               &      (21.4)   \\
\cmidrule{1-10}
\RSq                &        0.25   &        0.53   &        0.64   &        0.02   &        0.34   &        0.62   &        0.29   &        0.57   &        0.67   \\
Observations        &          39   &          39   &          39   &          39   &          39   &          39   &          39   &          39   &          39   \\
\Oster              &           .   &        -.59   &       -.045   &           .   &        -1.1   &        -.25   &           .   &         -61   &         -25   \\
Baseline controls   &           -   &         Yes   &         Yes   &           -   &         Yes   &         Yes   &           -   &         Yes   &         Yes   \\
   \bottomrule
