# Supplementary material for: Pandemics Depress the Economy, Public Health Interventions Do Not: Evidence from the 1918 Flu
Source: arXiv:2207.11636 source file (2022-07-24)
Supplement: Supplementary file 19 [file mortality_markel_peak_value_drop_west.tex]

&         (1)   &         (2)   &         (3)   &         (4)   &         (5)   &         (6)   &         (7)   &         (8)   &         (9)   \\
\cmidrule{1-10}Intensity&       -0.62***&       -0.60***&       -0.23   &               &               &               &               &               &               \\
                    &      (0.13)   &      (0.17)   &      (0.17)   &               &               &               &               &               &               \\
Speed               &               &               &               &       -0.97   &       -1.06   &       -0.42   &               &               &               \\
                    &               &               &               &      (0.98)   &      (0.96)   &      (0.77)   &               &               &               \\
High NPI            &               &               &               &               &               &               &      -57.49***&      -59.45***&      -36.12*  \\
                    &               &               &               &               &               &               &     (11.66)   &     (15.30)   &     (18.89)   \\
\cmidrule{1-10}
\RSq                &        0.25   &        0.53   &        0.64   &        0.02   &        0.34   &        0.62   &        0.29   &        0.57   &        0.67   \\
Observations        &          39   &          39   &          39   &          39   &          39   &          39   &          39   &          39   &          39   \\
\Oster              &           .   &        -.59   &       -.045   &           .   &        -1.1   &        -.25   &           .   &         -61   &         -25   \\
Baseline controls   &           -   &         Yes   &         Yes   &           -   &         Yes   &         Yes   &           -   &         Yes   &         Yes   \\
   \bottomrule
